# Supplementary material for: Zero-Shot Video Restoration and Enhancement with Assistance of Video Diffusion Models
Source: arXiv:2601.21922 source file (2026-11-18)
Supplement: Supplementary file 1 [file supplement.tex]

\documentclass{article} % For LaTeX2e
\usepackage{iclr2026_conference,times}

% Optional math commands from https://github.com/goodfeli/dlbook_notation.
\input{math_commands.tex}

\usepackage{hyperref}
\usepackage{url}

\usepackage{graphicx}
\usepackage[algo2e]{algorithm2e} 
\usepackage{multirow} 
\usepackage{booktabs}       % professional-quality tables
\usepackage{amsfonts}       % blackboard math symbols
\usepackage{nicefrac}       % compact symbols for 1/2, etc.
\usepackage{microtype}      % microtypography
\usepackage{xcolor}         % colors

\usepackage{amsthm,amsmath,amssymb}
\usepackage{mathrsfs}
\usepackage{threeparttable}
\usepackage{bigstrut}
\usepackage{float}

\usepackage{amsthm,amsmath,amssymb}
\usepackage{mathrsfs}

\usepackage{algorithm}
\usepackage{algorithmic}
\usepackage[algo2e]{algorithm2e} 
\usepackage{amsmath}

\usepackage{wrapfig} 
\usepackage{caption}

\title{Zero-Shot Video Restoration and Enhancement with Assistance of Video Diffusion Models \\ -- Supplementary Material --}

% Authors must not appear in the submitted version. They should be hidden
% as long as the \iclrfinalcopy macro remains commented out below.
% Non-anonymous submissions will be rejected without review.

\author{
    Cong Cao\textsuperscript{\rm 1},
    Huanjing Yue\textsuperscript{\rm 1},
    Shangbin Xie\textsuperscript{\rm 1},
    Xin Liu\textsuperscript{\rm 2},
    Jingyu Yang\textsuperscript{\rm 1} \\
\textsuperscript{\rm 1}School of Electrical and Information Engineering, Tianjin University, Tianjin, China\\
\textsuperscript{\rm 2}Computer Vision and Pattern Recognition Laboratory, School of Engineering Science, \\ Lappeenranta-Lahti University of Technology LUT, Lappeenranta, Finland\\
\texttt{\scriptsize{\{caocong\_123, huanjing.yue, chuancyx\}@tju.edu.cn, linuxsino@gmail.com, yjy@tju.edu.cn}}  \\
}

% The \author macro works with any number of authors. There are two commands
% used to separate the names and addresses of multiple authors: \And and \AND.
%
% Using \And between authors leaves it to \LaTeX{} to determine where to break
% the lines. Using \AND forces a linebreak at that point. So, if \LaTeX{}
% puts 3 of 4 authors names on the first line, and the last on the second
% line, try using \AND instead of \And before the third author name.

\iclrfinalcopy % Uncomment for camera-ready version, but NOT for submission.
\begin{document}

\maketitle

This supplementary file provides details that were not presented in the main paper due to page limitations. In the following, we first provide the details of the experiment settings. Then we present more comparison results. Hereafter, we provide an ablation study on the fusion ratio strategy. Finally, a demo for comparing video results is given. 

\section{Experiment Settings}

For the video restoration tasks, we add zero-shot video deblurring for comparison. Following \cite{cao2024zero}, we collected 10 ground truth (GT) videos from the dataset REDS \cite{nah2019ntire}. For the degradation of video deblurring, we follow \cite{kwon2024solving,kwon2024vision} and use the temporal uniform blur kernel. For all diffusion models, the prompts are null texts. The $M$ in COT-Based Fusion Ratio Strategy is set to 4. To accelerate the inference time, we apply the strategy every 10 timesteps and then apply the obtained $\lambda^{F1}$, $\lambda^{F2}$ and $\lambda^{F}$ to the following 9 timesteps. Our method can be combined with the aggregation sampling in \cite{wang2024exploiting} to test on higher-resolution videos. For long video, we separate it into different video clips, neighbouring video clips share one overlapping frame. When our Temporal-Strengthening Post-Processing finishes the process of the previous video clip, the last/shared frame is used as the image condition in the next video clip to maintain the long-range temporal consistency. All experiments were conducted on a 96G H20 GPU.

\section{Comparison with State-of-the-art Methods}

For zero-shot video deblurring, we compare our method with supervised (sup.) method VRT \cite{liang2024vrt} and zero-shot video restoration method SVI \cite{kwon2024solving} and VISION-XL \cite{kwon2024vision}. Since SVI only releases the code for zero-shot video deblurring, we do not compare it on other restoration tasks. Table \ref{ComparisonVDB} lists the quantitative results on the evaluation data for zero-shot video deblurring. It can be observed that our method outperforms the compared SOTA methods on all six metrics.

We also conducted a user study to further evaluate the visual quality and temporal consistency. To facilitate the comparison, we only compared the zero-shot video super-resolution results of PSLD, VISION-XL, and PSLD+ZVRV on eight groups of videos. Each user is asked to evaluate the visual quality and temporal consistency of the video with a score ranged from 1 to 3, where 3 indicates good
quality and 1 indicates bad quality. The average score for PSLD, VISION-XL, and PSLD+ZVRV is 2.07, 1.05 and 2.91, respectively, which demonstrates that our method has much better visual quality and temporal consistency. We also provide a demo video in the supplementary materials. 

The inference time of our method is contingent upon that of the employed T2V and I2V models. In the future, we will explore acceleration techniques for T2V and I2V models to expedite our method.

\begin{table}[t]
\centering
\caption{Quantitative comparison with state-of-the-art methods for zero-shot video deblurring. The best results are highlighted in bold and the second best results are underlined. The WE and t-LPIPS values have been multiplied by 100.}
%\begin{tabular}{m{5cm}m{0.7cm}<{\centering}m{0.7cm}<{\centering}}
%\begin{tabular}{m{2.2cm}m{1.0cm}<{\centering}m{0.9cm}<{\centering}m{0.9cm}<{\centering}m{0.9cm}<{\centering}m{0.9cm}<{\centering}m{0.9cm}<{\centering}m{0.9cm}<{\centering}}
\resizebox{0.8\textwidth}{11.5mm}{
\addtolength{\tabcolsep}{-5pt}
\begin{tabular}{l|c|c|c|c|c|c|c|c|c|c}
%\begin{tabular}{m{5cm}m{0.7cm}m{0.7cm} }
%\begin{tabular}
\toprule
Methods              & Backbone  & PSNR$\uparrow$  & SSIM$\uparrow$  & CLIP-IQA$\uparrow$ & LPIPS$\downarrow$ & WE$\downarrow$ & FVD$\downarrow$ & DOVER$\uparrow$ & t-LPIPS$\downarrow$ & VMAF$\uparrow$\\
\hline
VRT(sup.)	         & - &18.98 &0.4505 &0.2093 &0.7155 &\underline{0.1816} &1694.8 & \underline{7.581} & \underline{0.86} & \underline{81.94} \\
\hline
PSLD                 & SDXL &19.69	&0.4996	&0.1905	&0.4546	&1.5298	&662.0  & 5.573 & 3.12 & 76.02\\
SVI                  & -    &18.25	&0.4839	&0.2010	&0.5871	&1.3463	&1218.3 & 7.202 & 2.35 & 79.47 \\
VISION-XL	         & SDXL &\underline{19.82}	&\underline{0.5068}	&\underline{0.2147}	&\underline{0.4232}	&1.2623	&\underline{457.7} & 7.298 &1.84 & 80.66\\
PSLD+ZVRV	         & SDXL &\textbf{20.47}	&\textbf{0.5342} &\textbf{0.4813} &\textbf{0.3675}	&\textbf{0.1632} &\textbf{326.4} & \textbf{8.456} & \textbf{0.67} & \textbf{84.53} \\
\bottomrule
\end{tabular}
}
\label{ComparisonVDB}
\end{table}

\section{Ablation Study}

\begin{table}
\centering
\caption{Ablation study on the COT-based fusion ratio strategy (with different hyperparameters $M$ and $r$) and the fixed fusion ratio strategy. The best results are highlighted in bold.}
\resizebox{0.99\textwidth}{12mm}{
\begin{tabular}{ccc|c|c|c|c|c|c|c|c}
\toprule
\multicolumn{2}{l}{Fusion Ratio Strategy}                  & PSNR$\uparrow$  & SSIM$\uparrow$  & CLIP-IQA$\uparrow$ & LPIPS$\downarrow$ & WE$\downarrow$ & FVD$\downarrow$ & DOVER$\uparrow$ & t-LPIPS$\downarrow$ & VMAF$\uparrow$\\
\hline
\multirow{5}{*}{COT-Based Fusion Ratio Strategy} &$M$=2, $r$=0.45  &26.74  &0.6953	&0.8472 &0.1649  &0.4186  &258.5 & 7.251 & 0.92 & 83.42    \\\cline{2-11}
                                                 &$M$=3, $r$=0.45  &27.15  &0.7196	&0.8599 &0.1573  &0.3952  &240.8 & 8.854 & 0.63 & 85.01    \\\cline{2-11}
                                                 &$M$=4, $r$=0.45  &\textbf{27.42}  &\textbf{0.7388} &\textbf{0.8691} &\textbf{0.1395}  &\textbf{0.3755}  &\textbf{231.7} & \textbf{9.076} & \textbf{0.41} & \textbf{86.37}    \\\cline{2-11}
                                                 &$M$=4, $r$=0.50  &27.20  &0.7316	&0.8610 &0.1432  &0.3764  &239.5 & 8.983 & 0.51 & 86.04    \\\cline{2-11}
                                                 &$M$=4, $r$=0.40  &27.09  &0.7272	&0.8623 &0.1408  &0.3783  &234.1 & 8.779 & 0.50 & 85.79    \\\hline
\multicolumn{2}{l}{Fixed Fusion Ratio Strategy}                &26.59  &0.6915	&0.8347 &0.1724  &0.4298  &265.2 & 6.451 & 0.98 & 82.26\\
\bottomrule
\end{tabular}
}
\label{Ablation}
\end{table}

In this section, we conduct an ablation study on the COT-based fusion ratio strategy (with different hyperparameters \( M \) and \( r \)) and the fixed fusion ratio strategy. For the fixed fusion ratio strategy, we set \( \lambda^{F1} \), \( \lambda^{F2} \), and \( \lambda^{F} \) to 0.1, 0.01, and 0.5, respectively, for all timesteps.. For hyperparameter \( r \), the value is halved after each search. Taking 4$\times$ blind video super-resolution as an example, Table \ref{Ablation} lists the quantitative comparison results. It can be observed that the COT-based fusion ratio strategy is more sensitive to the hyperparameter \( M \). As \( M \) increases, the performance improves as well. Considering the trade-off between speed and performance, we set \( M = 4 \), and we set \( r = 0.45 \) since it achieves the best performance when \( M = 4 \). Besides, we apply the COT-based fusion ratio every 10 timesteps and apply the obtained $\lambda^{F1}$, $\lambda^{F2}$, and $\lambda^{F}$ to the following 9 timesteps. Although applying the COT-based fusion ratio more frequently can result in better performance, we choose to apply it every 10 timesteps considering the trade-off between speed and performance. When \( M \) ranges from 2 to 4, and \( r \) ranges from 0.4 to 0.5, the COT-based fusion ratio strategy consistently outperforms the fixed fusion ratio strategy.

%\appendix
%\section{Appendix}
%You may include other additional sections here.

\bibliography{iclr2026_conference_supp}
\bibliographystyle{iclr2026_conference}

\end{document}
